# Supplementary material for: A Gauss-Newton method for iterative optimization of memory kernels for generalized Langevin thermostats in coarse-grained molecular dynamics simulations
Source: arXiv:2402.10652 ancillary file (2024-06-21)
Supplement: Supplementary file 1 [file SM.pdf]

# Supplemental Material for "A Gauss-Newton method for iterative optimization of memory kernels for generalized Langevin thermostats in coarse-grained molecular dynamics simulations"

Viktor Klippenstein, Niklas Wolf, and Nico F. A. van der Vegt
*Department of Chemistry, Technical University of Darmstadt, 64287 Darmstadt, Germany*

(*Electronic mail: vandervegt@cpc.tu-darmstadt.de)

(*Electronic mail: wolf@cpc.tu-darmstadt.de)

(*Electronic mail: klippenstein@cpc.tu-darmstadt.de)

## S1. CORRELATION FUNCTIONS FROM THE PREPARATORY STEP AND THERMOSTAT MEMORY KERNELS

As shown in Fig. 1, the application of IOMK and IOMK-GN requires a preparatory step to evaluate $C_{VV}^{\mathrm{tgt}}(t)$, $C_{VV}^{\circ}(t)$, $G^{\mathrm{tgt}}(t)$ and $G^{\circ}(t)$, which are shown in Fig. S1 a)-b) for the studied ethanol system and the corresponding IBI model. We also compare the final thermostat memory kernel (12th iteration) from the IOMK and IOMK-GN methods. Both methods quantitatively converge to the same result. Note that on short time scales, the final memory kernel and the initial guess $(G^{\mathrm{tgt}} - G^{\circ}(t))$ are in perfect agreement, as already indicated by the fact that the 0th iteration in Fig. 2 shows good agreement on short time scales. Accordingly, $G^{\mathrm{tgt}} - \tilde{G}^{\mathrm{IOMK\text{-}GN}}$, which represents the memory kernel due to the conservative interaction in the final aux-GLE model, and $G^{\circ}(t)$ coincide on short time scales. This means that the CG DoFs and the DoFs removed in the coarse-graining process are not strongly coupled on short timescales, which is the reason why the initial guess applied in Sec. IV already yields accurate dynamics on short timescales.

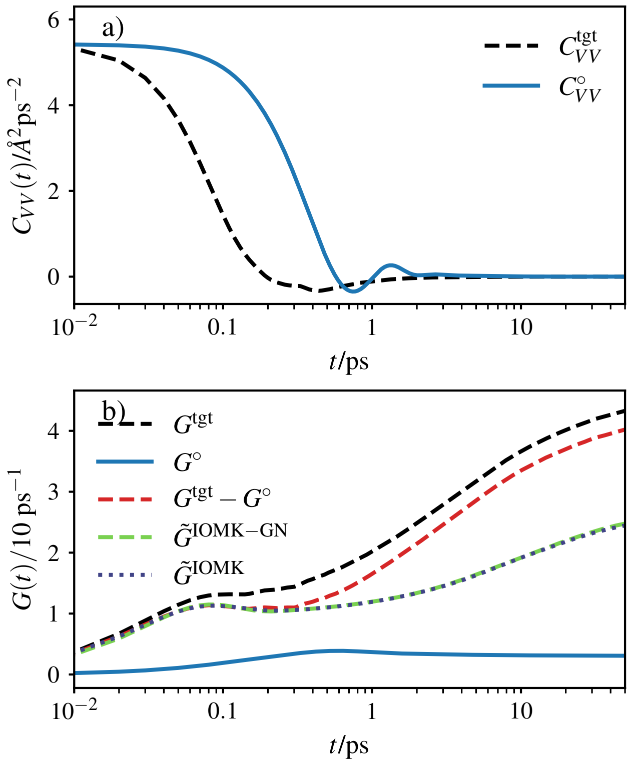


FIG. S1. a) The atomistic COM VACF ($C_{VV}^{\mathrm{tgt}}$) and the VACF from CG-MD simulations ($C_{VV}^{\circ}$). b) Comparison of several integrated memory kernels. $\tilde{G}^{\mathrm{IOMK\text{-}GN}}$ and $\tilde{G}^{\mathrm{IOMK}}$ represent the thermostat memory kernel of the 12th iteration of IOMK-GN and IOMK, respectively.

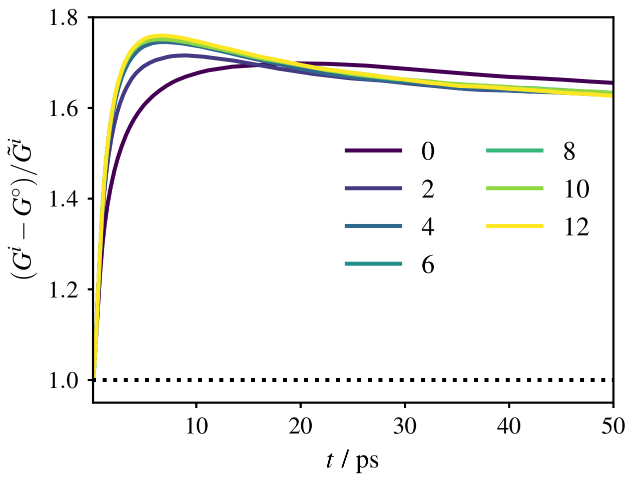


FIG. S2. The proportionality factor of the IOMK method (Eq. 19) evaluated for a set of iterations of the IOMK-GN method as presented in Fig. 2.

## S2. LINEAR RELATION BETWEEN THERMOSTAT AND SINGLE-PARTICLE MEMORY KERNEL

The reason why IOMK converges rapidly, and the Jacobian for the IOMK-GN method can be accurately and efficiently approximated without running CG simulations for every partial derivative is based on the linear approximation Eq. 19. Currently, there is no rigorous justification for assuming this linearity. In Ref. 1, we motivated the approach by observing that a similar relationship holds for different contributions to single-particle memory kernels between different systems. In Ref. 2, we have demonstrated through numerical experiments that in CG models, when using a Markovian Langevin thermo-

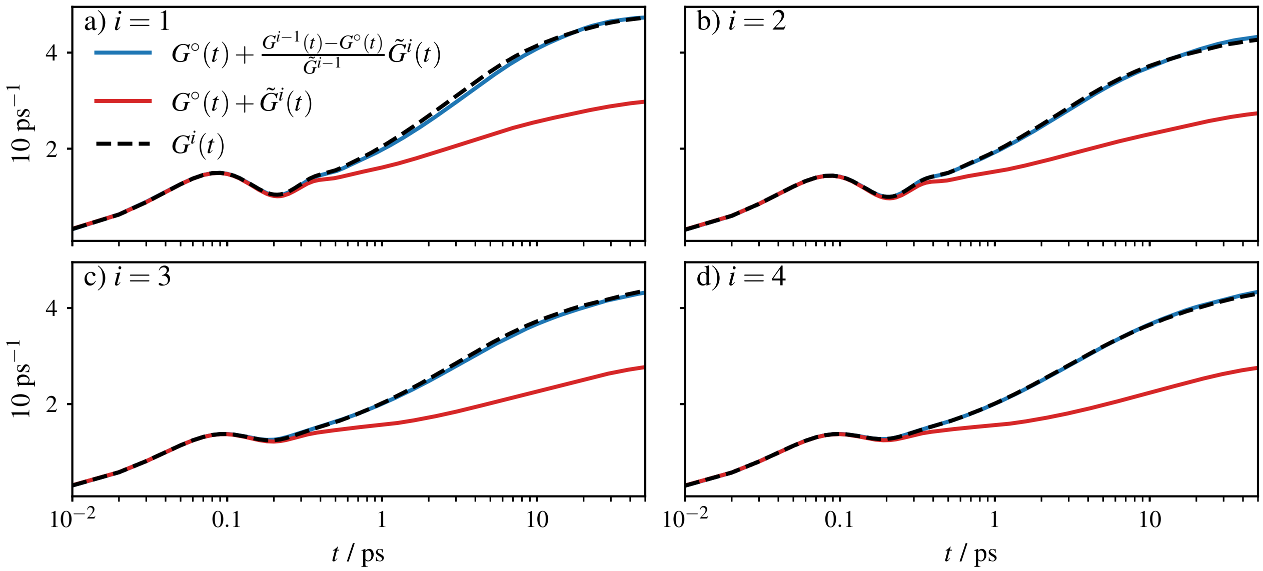


FIG. S3. Comparison of the total integrated memory kernel (black dashed line) to the prediction due to Eq. 19 (blue line) for the first four iterations of the IOMK-GN method presented in Fig. 2. For reference, the prediction from additivity is also shown (red line).

stat, the friction induced by conservative interactions depends linearly on the friction parameter in the thermostat.

Eq. 18 presumes a linear relation between the total integrated memory kernel $G^i(t)$ and the integrated memory kernel of the thermostat $\tilde{G}^i(t)$. With Eq. 19 we thus assume that the proportionality factor $(G^{i-1}(t) - G^\circ(t))/\tilde{G}^{i-1}(t)$ is independent of $\tilde{G}^{i-1}(t)$. This is, of course, not necessarily strictly true, but its local reevaluation in each iteration corrects for minor non-linearities.

In Fig. S2, we show the proportionality factor for some iterations derived from the same data shown in Fig. 2. As expected, the proportionality factor is not strictly constant over all iterations; otherwise, IOMK would always converge within a single iteration.

One could naively assume that the integrated thermostat memory kernel $\tilde{G}(t)$ contributes additively to the integrated total memory kernel $G(t)$. The lines then would all collapse on a horizontal line at one. Compared to this assumption, the variations of the proportionality factor over the iterations are clearly within a small range and, thus, generally give a reasonable estimate.

In Fig. S3 we compare the prediction Eq. 19 makes for $G^i(t)$ with the actual measurement by Eq. 7 for the first 4 iterations of IOMK-GN (see Sec. IV). Eq. 19 gives a substantial improvement over the naive assumption of additivity and is in quantitative agreement with the measured results.

## S3. EFFICIENT EVALUATION OF TIME-DEPENDENT MATRIX EXPONENTIALS

Linking a drift matrix to a memory kernel through Eqs. 5 or 22 suggests that a matrix exponential must be evaluated for each discretized point in time. When many partial derivatives have to be evaluated to calculate a Jacobian, this has implications that need to be considered in numerical implementations:

The matrix exponential in Eq. 22 can be expressed in terms of its series expansion

$$e^{-|t|\boldsymbol{A}_{ss}} = \sum_{k=0}^{\infty} \frac{1}{k!} (-|t|)^k \boldsymbol{A}_{ss}^k. \tag{S1}$$

For small $t$, the series expansion can be truncated after the first few powers. In the examples considered in this work, $t$ spans four orders of magnitude, which prohibits the use of Eq. S1. Well-established linear algebra libraries, such as SciPy[3], implement more reliable algorithms for computing matrix exponents.

However, to evaluate a single Jacobian for $\mathscr{M}$ discretized points in time and $\mathscr{N}$ parameters involves at least $\mathscr{N} \times \mathscr{M}$ (which amounts to $5000 \times 44 = 2 \cdot 10^5$ in the examples discussed in the main text) evaluations of matrix exponentials per GN iteration. If done naively, this can result in significant computational overhead. For equidistantly discretized memory kernels, the computation can be significantly accelerated by considering

$$\boldsymbol{H}_m = e^{-m|\Delta t|\boldsymbol{A}_{ss}} = \left(e^{-|\Delta t|\boldsymbol{A}_{ss}}\right)^m = \boldsymbol{H}_{m-1}\boldsymbol{H}_1 \tag{S2}$$

and thus only a single matrix exponential has to be calculated in each evaluation of Eq. 22, and with $\boldsymbol{H}_0 = \boldsymbol{I}$ and $\boldsymbol{H}_1 = \exp\{-|\Delta t|\boldsymbol{A}_{ss}\}$, Eq. S2 can be evaluated iteratively. We can further note, that $\boldsymbol{H}_m$ for $m \geq 2$ can also be evaluated by

$$\boldsymbol{H}_m = \boldsymbol{H}_{\lfloor m/2 \rfloor} \boldsymbol{H}_{\lfloor (m+1)/2 \rfloor}, \tag{S3}$$

where $\lfloor\,\rfloor$ denotes the floor function. Since in Eq. S3 matrix multiplications are always performed with matrices of similar

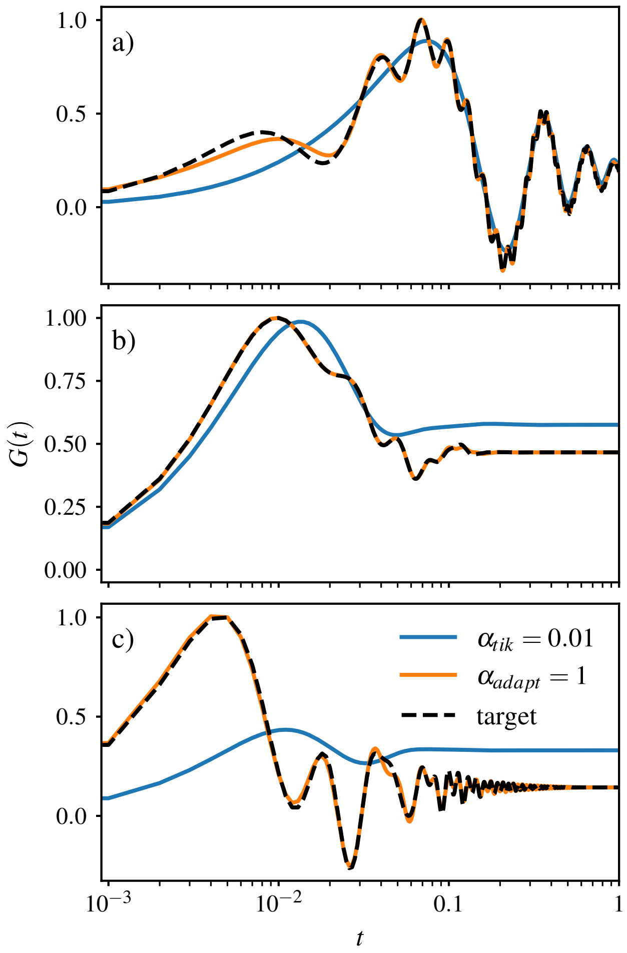


FIG. S4. Fits to three exemplary randomly generated integrated memory kernels (see Sec. S4 A) with $\alpha_{\rm tik} = 0.01$ and $\alpha_{\rm adapt} = 1$.

power of $\boldsymbol{H}_1$, we expect smaller rounding errors compared to Eq. S2.

With this approach, the evaluation of the Jacobian in one GN iteration involves approximately $\mathcal{N} \times \mathcal{M}$ matrix multiplications of $h \times h$, which is efficient compared to evaluating $\mathcal{N} \times \mathcal{M}$ matrix exponentials.

## S4. COMPARING REGULARIZATION SCHEMES FOR FITTING OF MEMORY KERNELS

### A. Generation and fitting of random memory kernels

This section describes how the data shown in Fig. 4 was generated. We considered 100 integrated memory kernels of the form

$$G(t) = \sum_{k=1}^{4} \left( \frac{e^{-0.5 a_k x}}{(a_k^2 + 4d_k^2)} ((-2a_k b_k - 4c_k d_k) cos(d_k x) + (-2a_k c_k + 4 b_k d_k) sin(d_k x)) - (-2a_k b_k - 4 c_k d_k) \right)$$

which can be represented in the aux-GLE by the drift matrix[4]

$$\boldsymbol{A} = \begin{pmatrix} 0 & (\boldsymbol{A}_{ps})_1^T & (\boldsymbol{A}_{ps})_2^T & (\boldsymbol{A}_{ps})_3^T & (\boldsymbol{A}_{ps})_4^T \\ -(\boldsymbol{A}_{ps})_1 & (\boldsymbol{A}_{ss})_{11} & \mathbf{0} & \mathbf{0} & \mathbf{0} \\ -(\boldsymbol{A}_{ps})_2 & \mathbf{0} & (\boldsymbol{A}_{ss})_{22} & \mathbf{0} & \mathbf{0} \\ -(\boldsymbol{A}_{ps})_3 & \mathbf{0} & \mathbf{0} & (\boldsymbol{A}_{ss})_{33} & \mathbf{0} \\ -(\boldsymbol{A}_{ps})_4 & \mathbf{0} & \mathbf{0} & \mathbf{0} & (\boldsymbol{A}_{ss})_{44} \end{pmatrix} \tag{S4}$$

with

$$(\boldsymbol{A}_{ps})_k^T = \left( \sqrt{\frac{b_k}{2} - \frac{c_k d_k}{a_k}}, \sqrt{\frac{b_k}{2} + \frac{c_k d_k}{a_k}} \right) \tag{S5}$$

and

$$(\boldsymbol{A}_{ss})_{kk} = \begin{pmatrix} a_k & \frac{1}{2}\sqrt{4d_k^2 + a_k^2} \\ -\frac{1}{2}\sqrt{4d_k^2 + a_k^2} & 0 \end{pmatrix}. \tag{S6}$$

We have constructed the random kernel in such a way that it can be represented in principle by the drift matrix defined above. To ensure that any set of parameters $(a_k, b_k, c_k, d_k)$ would yield real entries in $\boldsymbol{A}$, we introduce two additional variables $e_k$ and $f_k$ such that

$$c = \frac{a_k f_k - a_k e_k}{2d_k} \tag{S7}$$

$$b = 2e_k + 2\frac{c_k d_k}{a_k}. \tag{S8}$$

We drew four random numbers ($\xi_1$, $\xi_2$, $\xi_3$, $\xi_4$) per damped oscillator (16 per memory kernel) between 0 and 1 from a uniform distribution and set $a_k = 5 + 100\xi_1$, $e_k = \xi_2$, $f_k = \xi_3$, $d_k = 500\xi_4$. These parameters were used to generate discretized memory kernels up to $t_{\rm max} = 1$ with equidistant spacing $\Delta t = 0.001$.

Based on the set of random memory kernels (see Fig. 4), we determined that the optimal regularization parameter is $\alpha = 1$ for the adaptive scheme. While for the random memory kernels $\alpha = 1$ also yields the best results for the Tikhonov regularizations, we note that the random memory kernels typically have high frequency modes that are not present in the memory kernels of ethanol. Tests on smoother kernels show that the $\alpha = 0.01$ Tikhonov scheme performs slightly better for more realistic examples. In Fig. S4, we show three of the randomly generated kernels along with the corresponding fits. In all three cases, it can be seen that the adaptive regularization achieves good fits within 100 iterations. By contrast,

the Tikhonov regularization at best reproduces the qualitative structure (a and b) or fails to match any distinct features (c). Of course, these are extreme examples since the memory kernels we need to represent in the CG ethanol model are less noisy.

### B. Exemplary coarse-grained ethanol memory kernel fitting

For a more practical example, we also fit $G(t)$, $\tilde{G}^{IOMK-GN}(t)$ (the memory kernels generated by the optimized drift matrix of IOMK-GN), and $G^{\circ}(t)$, and show the results in Fig. S5. Here, the discrepancy between the two regularization schemes is not as dramatic, but still, the Tikhonov regularization fails to fit either the short time scales (a and b) or the long time scales (c). In Fig. S6, we show the change in average residuals with respect to iterations for the same test functions, using both regularization schemes with different regularization parameters. We find that the adaptive regularization with $\alpha = 1$ achieves orders of magnitude smaller residuals than the Tikhonov scheme for any regularization parameter. Note that the results shown are always the final fit after 100 iterations and thus do not indicate that the Tikhonov regularization cannot converge to more satisfactory results given more time. However, in terms of performance and reliability, the adaptive scheme is preferable for our purpose.

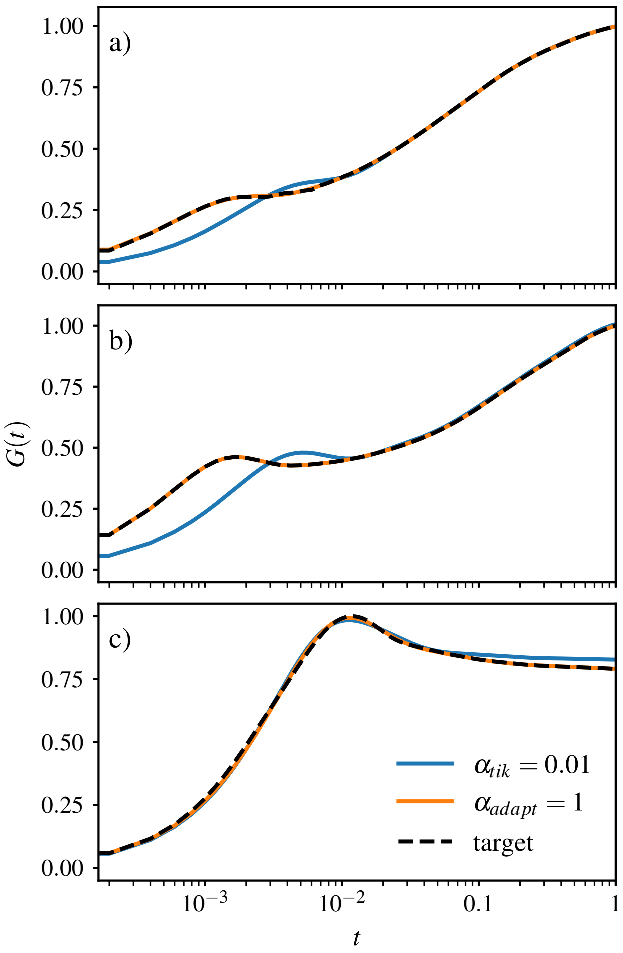


FIG. S5. a) $G^{\mathrm{tgt}}$, b) $\tilde{G}^{IOMK-GN}$ from the IOMK-GN results (see Sec. IV) and c) $G^{\circ}$ and the corresponding fits using the optimal regularization parameters $\alpha_{\mathrm{tik}} = 0.01$ and $\alpha_{\mathrm{adapt}} = 1$.

## S5. COMPARING ADAPTIVE AND TIKHONOV REGULARIZATION IN IOMK-GN

In the left column of Fig. 2, the results of the IOMK-GN method are summarized. Therein we applied the IOMK-GN method with an initial guess constructed from $\tilde{G}^0(t) = G^{\mathrm{tgt}} - G^{\circ}(t)$, using the adaptive regularization scheme with $\alpha_{\max} = 1$ and optimized the regularization parameter in every iteration as described in Appendix B 1. Results from fitting suggest that the adaptive regularization converges more quickly than Tikhonov. In Fig. S7, we compare the results from the main text with the Tikhonov regularization, where we used the same initial guess and the same regularization parameter optimization with $\alpha_{\max} = 0.01$. Contrary to the observations in Figs. S4, S5 and S6, the Tikhonov regularization seems to perform better as there is no distortion of the short time scales in the first iterations. When using the Tikhonov regularization, the short time scales are not altered, and the provided initial guess already allows for an accurate match of short time scales. Note however, that for generating the initial guess, we applied the adaptive regularization for fitting.

To compare the two regularization schemes in a more general setting, instead of deriving $\boldsymbol{A}^0$ from an initial guess of $\tilde{G}^0(t) = G^{\mathrm{tgt}} - G^{\circ}(t)$ one can also use an *a-priori* initial guess as suggested in Appendix B 4. Since the initial guess here is not directly informed by the dynamics of the FG model, it is far from optimal and cannot encode detailed short time scale dynamics. When using the adaptive regularization (Sec. II E) and the update step optimization (Appendix B 1), IOMK-GN still converges quickly to an optimal solution as shown in Fig. S8 a)-c). When the Tikhonov regularization is used instead, only the long-time dynamics are matched within 12 iterations, while further progress on the short-time dynamics is stalled. These results are consistent with tests performed by fitting memory kernels.

As a final test, we applied the IOMK-GN with the same setup as used in Fig. S8, but with a fixed regularization parameter (without optimization based of Eq. 18). On long time scales, IOMK-GN still yields an quantitative match within few iterations, while the short time dynamics converge slower. With the adaptive regularization there is still significant improvement. When using the proposed Gauss-Newton method for fitting, good results are typically achieved after $\approx 20$ iterations. Thus, we would expect that running more iterations would allow for a better match.

From the additional data in Figs. S7-S9, we conclude:

1. Using $\tilde{G}^0(t) = G^{\mathrm{tgt}} - G^{\circ}(t)$ to construct an initial guess $\boldsymbol{A}^0$ which captures features of the short time dynamics

2. The long time dynamics converge rapidly for both regularization schemes.

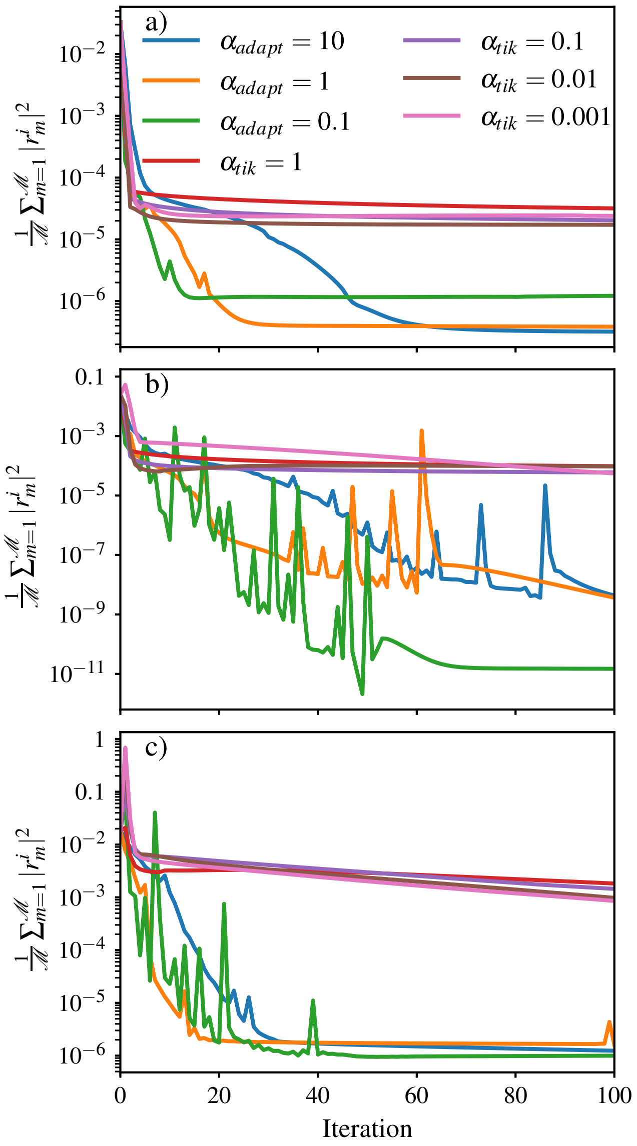


FIG. S6. Comparison of the averaged squared residuals for different regularization parameters for the data of Fig. S5 in order. The residuals are evaluated based on the normalized representation of the target memory kernel and drift matrix, as described in Appendix B 2.

3. The adaptive scheme performs better than the Tikhonov regularization when starting from a sub-optimal *a-priori* initial guess.

4. The optimization of the regularization parameter further speeds up convergence.

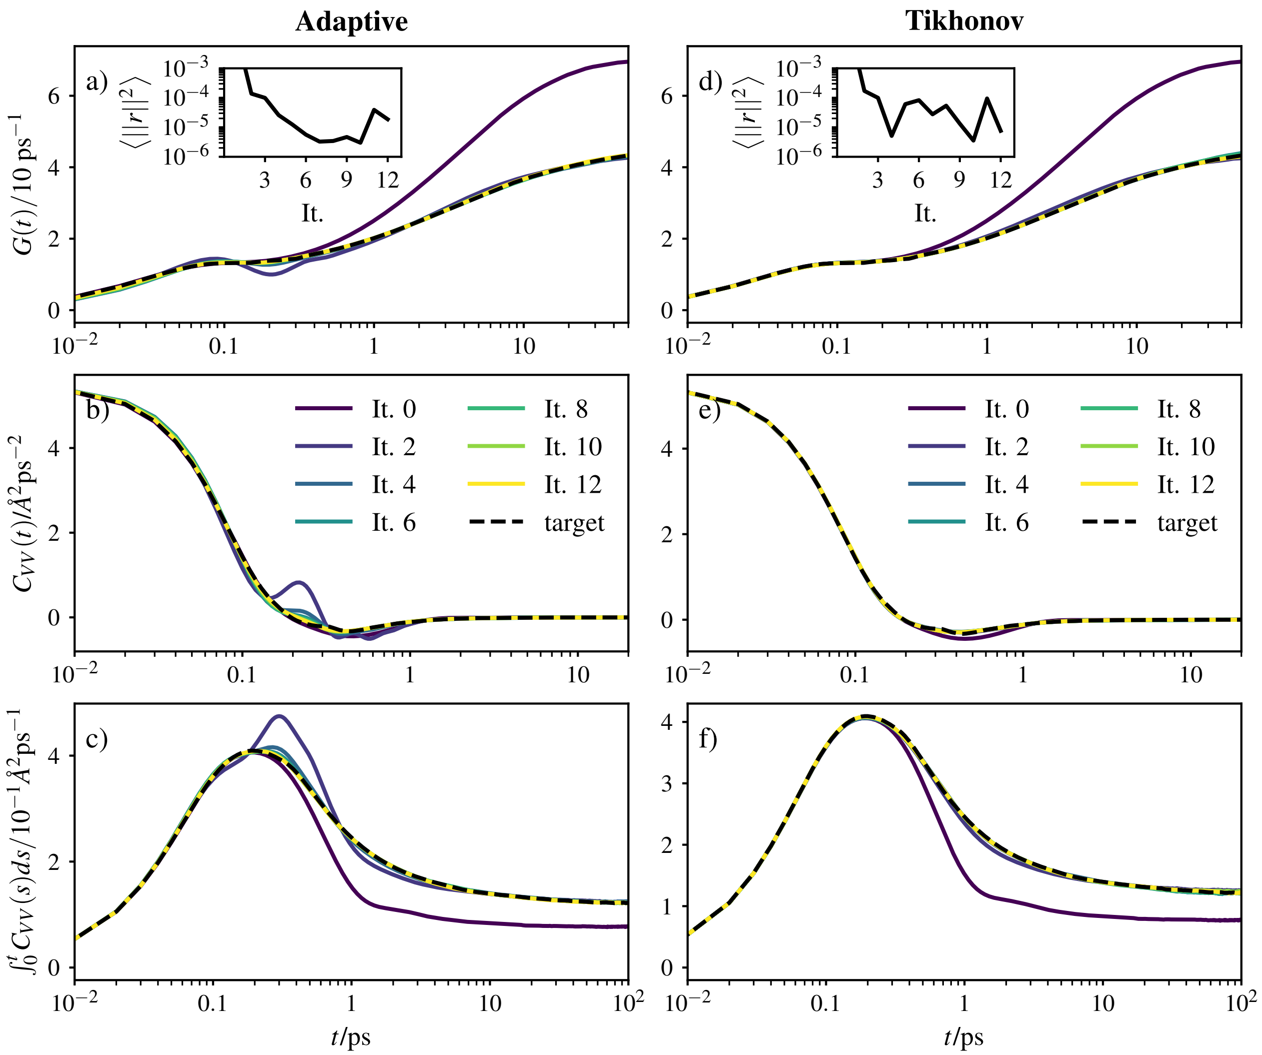


FIG. S7. Summary of the results for IOMK-GN with adaptive regularization and $\alpha_{\mathrm{max}} = 1$ (a-c) and Tikhonov regularization with $\alpha_{\mathrm{max}} = 0.01$ (d-f). The top, middle, and bottom rows show the integrated single particle memory kernel, the VACF, and the integrated VACF for a few selected iterations, compared to the respective target. The insets in a) and d) show the averaged squared residuals in the normalized representation.

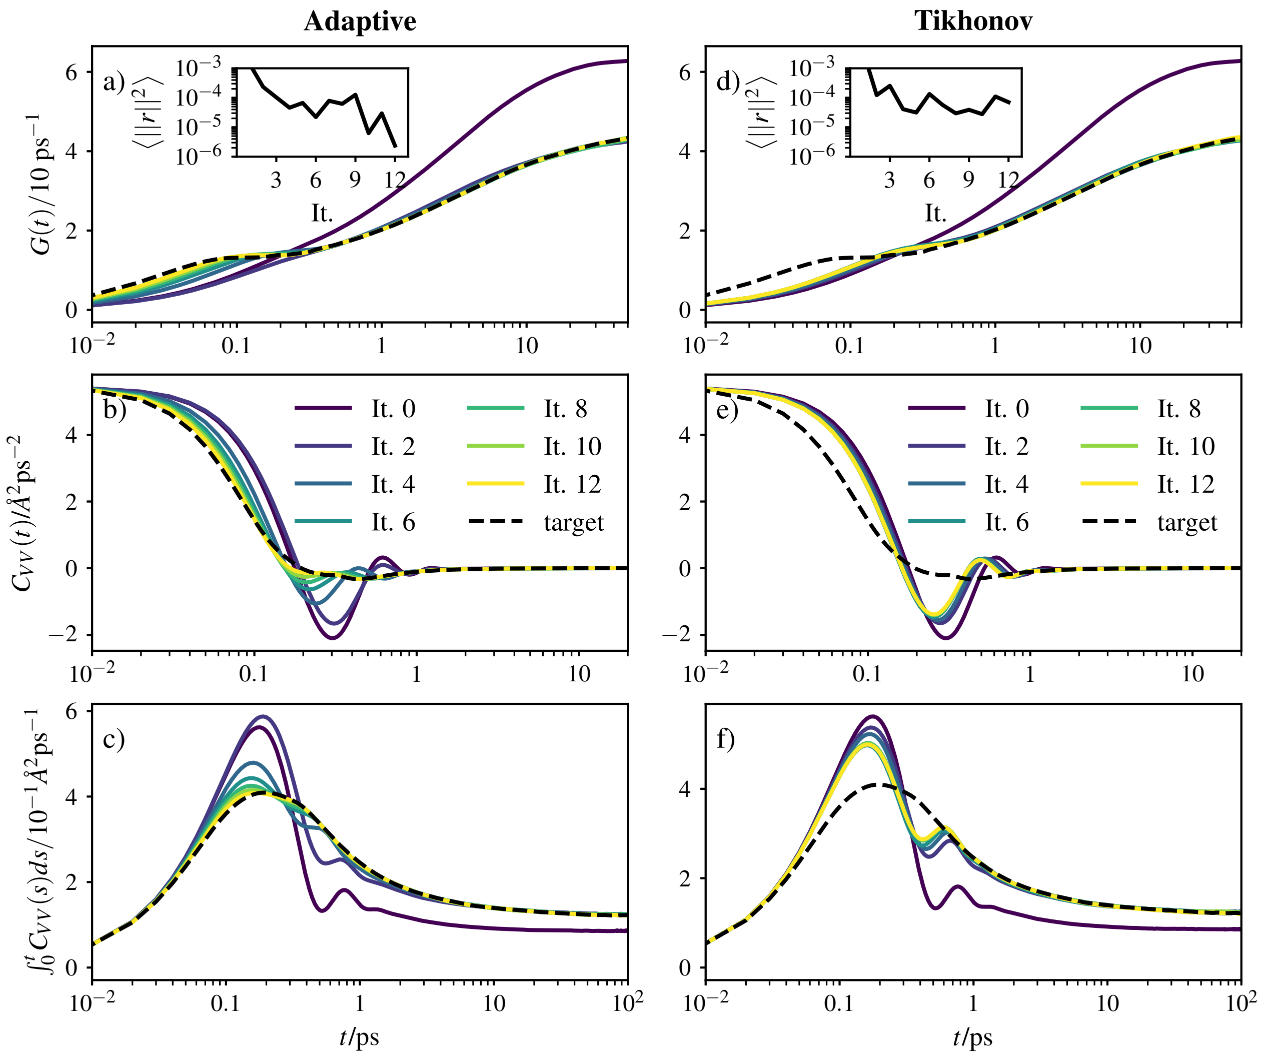


FIG. S8. Summary of the results for IOMK-GN with adaptive regularization and $\alpha_{\max} = 1$ (a-c) and Tikhonov regularization with $\alpha_{\max} = 0.01$ (d-f), using an initial guess as described in Appendix B 4. The top, middle, and bottom rows show the integrated single particle memory kernel, the VACF, and the integrated VACF for a few selected iterations, compared to the respective target. The insets in a) and d) show the averaged squared residuals in the normalized representation.

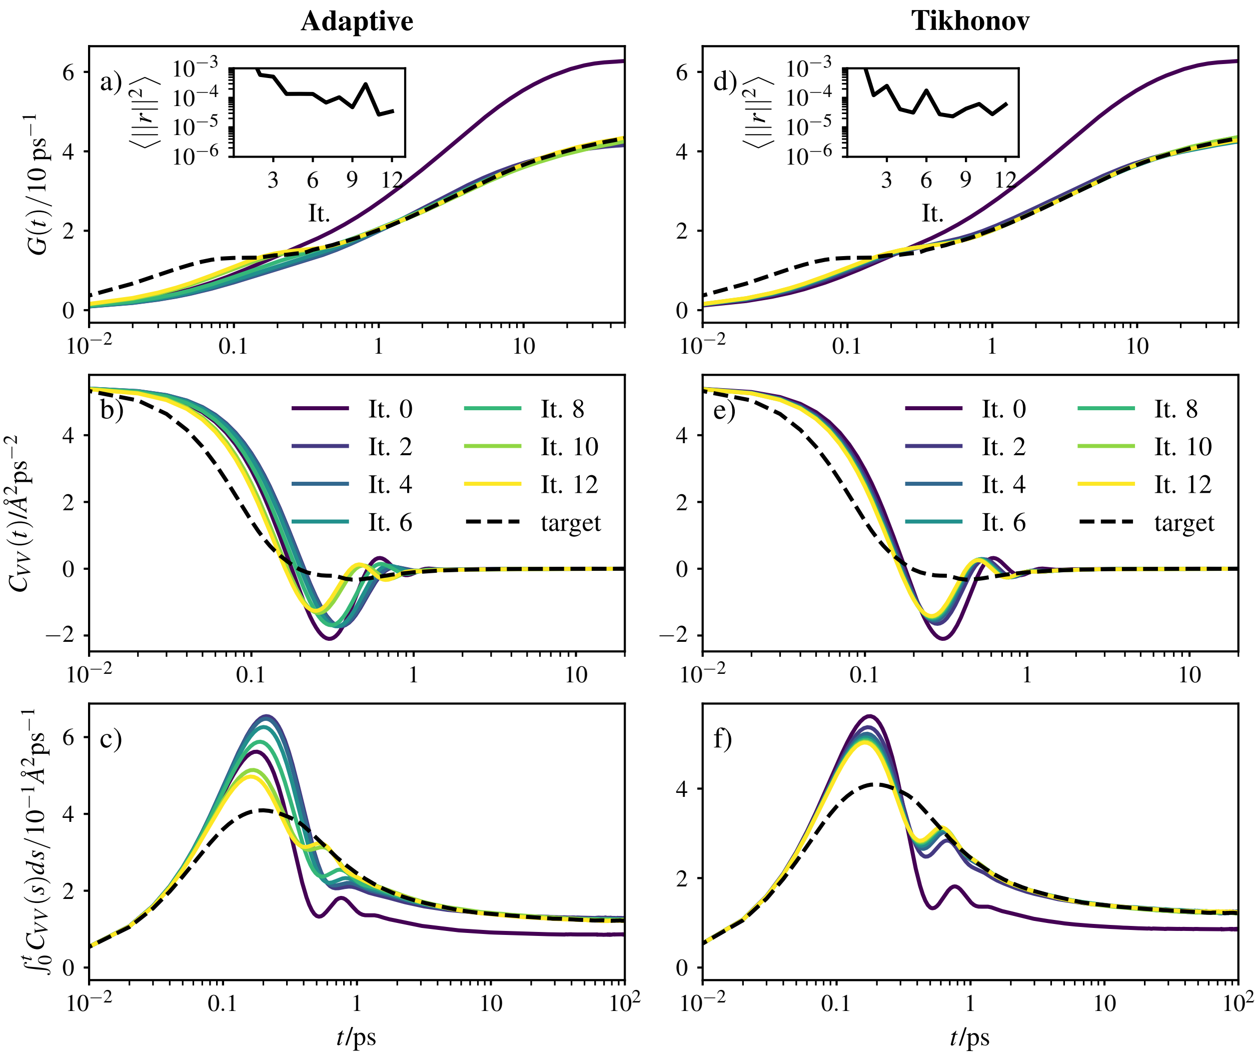


FIG. S9. Summary of the results for IOMK-GN with adaptive regularization and $\alpha = 1$(a-c) and Tikhonov regularization with $\alpha = 0.01$ (d-f), using an initial guess as described in Appendix B 4. Here, the regularization parameters were not optimized. The top, middle, and bottom rows show the integrated single particle memory kernel, the VACF, and the integrated VACF for a few selected iterations, compared to the respective target. The insets in a) and d) show the averaged squared residuals in the normalized representation.

[1] V. Klippenstein and N. F. A. van der Vegt, “Cross-correlation corrected friction in generalized Langevin models: Application to the continuous Asakura–Oosawa model,” The Journal of Chemical Physics **157**, 044103 (2022).
[2] V. Klippenstein and N. F. A. van der Vegt, “Bottom-Up Informed and Iteratively Optimized Coarse-Grained Non-Markovian Water Models with Accurate Dynamics,” Journal of Chemical Theory and Computation **19**, 1099–1110 (2023).
[3] P. Virtanen, R. Gommers, T. E. Oliphant, M. Haberland, T. Reddy, D. Cournapeau, E. Burovski, P. Peterson, W. Weckesser, J. Bright, S. J. van der Walt, M. Brett, J. Wilson, K. J. Millman, N. Mayorov, A. R. J. Nelson, E. Jones, R. Kern, E. Larson, C. J. Carey, İ. Polat, Y. Feng, E. W. Moore, J. VanderPlas, D. Laxalde, J. Perktold, R. Cimrman, I. Henriksen, E. A. Quintero, C. R. Harris, A. M. Archibald, A. H. Ribeiro, F. Pedregosa, and P. van Mulbregt, “SciPy 1.0: Fundamental algorithms for scientific computing in Python,” Nature Methods **17**, 261–272 (2020).
[4] S. Wang, Z. Li, and W. Pan, “Implicit-solvent coarse-grained modeling for polymer solutions via Mori-Zwanzig formalism,” Soft matter **15**, 7567–7582 (2019).
